# Supplementary material for: Xinyu AI Search: Enhanced Relevance and Comprehensive Results with Rich Answer Presentations
Source: arXiv:2505.21849 source file (2025-05-28)
Supplement: Supplementary file 1 [file expansion.tex]

\subsection{Query Expansion}
\label{app:expansion}
